# Supplementary material for: On the Robustness of Bayesian Neural Networks to Adversarial Attacks
Source: arXiv:2207.06154 source file (2024-02-28)
Supplement: Supplementary file 1 [file Supplementary.tex]

%\section{Further Results}

%In what follows we present additional empirical results: in Section \ref{sec:multimodality} we add an experimental justification for Remark \ref{remark_bernstein}, while in Section \ref{sec:deep_ensembles} we examine the relationship between BNNs and Deep Ensemble architectures.

\iffalse
\subsection{Multimodal posterior distributions}
\label{sec:multimodality}
Figure \ref{fig:multimodality} empirically confirms remark \ref{remark_bernstein} \ap{Remark doesn't exist anymore}, by showing that for MNIST the posterior distributions of the weights are multimodal. %, thus Bernstein von Mises theorem does not apply to BNNs.
\begin{figure}[!ht]
\centering
\includegraphics[width=0.75\columnwidth]{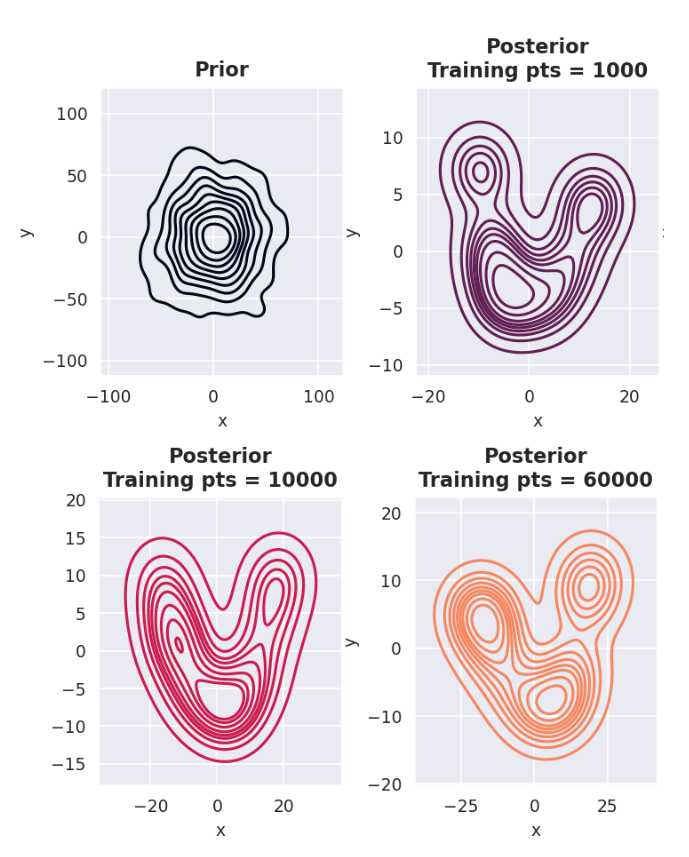}
\caption{Prior and posterior distributions for models trained with an increasing number of training points. Models are trained on MNIST dataset with HMC.  Samples are projected on the first two principal components (here $x$ and $y$) using PCA. %\LL{What are x and y axis?}\gc{the first two principal components}
}
\label{fig:multimodality}
\end{figure}
\fi

\subsection{Comparison with Deep Ensembles}
\label{sec:deep_ensembles}

\section{Training hyperparameters for BNNs}
\label{sec:training_hyperparams}
Tables \ref{table:half_moons_hmc.}, \ref{table:MNIST_hmc}, \ref{table:MNIST_VI} and \ref{table:MNIST_SGD} summarize the sets of hyperparameters used to tune our models. BNNs' architectures achieving the highest test accuracy are described in Table \ref{table:bnns_hmc} for HMC training and \ref{table:bnns_vi} for VI training.
